# Supplementary material for: Output-Sensitive Adaptive Metropolis-Hastings for Probabilistic Programs
Source: arXiv:1501.05677 source file (2015-05-05)
Supplement: Supplementary file 1 [file appendix.tex]

\section{Appendix}

\subsection{Analysis of $B(p_1)$}

The right-hand side of (\ref{eqn:lemma-rate-equilibrium}) is
\begin{equation}
	B(p_1)=\frac {1+\frac {p_1 \log p_1} {1-p_1}} {\frac 1 {p_1}+\frac {p_1 \log p_1} {1-p_1}}
	\label{eqn:appendix-B}
\end{equation}
We will show that the function is monotonous and defined
everywhere in $p_1 \in [0, 1]$. The function is immediately
defined for $p_1 \in (0, 1)$, because both the numerator and the
denominator are defined, and the denominator is not equal to
zero. To determine the values of $B(p_1)$ for $p_1=0$ and
$p_1=1$, we shall compute the limits of $B(p_1)$ at these
values (for example, using Maxima~\cite{maxima}). 
\begin{align}
	\lim_{p_1\to 0} B(p_1)& = 0\nonumber\\
	\lim_{p_1\to 1} B(p_1)& = \frac 1 3
	\label{eqn:appendix-B-limits}
\end{align}
It now remains to show that $B(p_1)$ is monotonic for $p_1 \in
(0, 1)$. One can use Maxima again (or perform the derivations
manually) to obtain $\frac {dB(p_1)} {dp_1}$ symbolically and
verify that it is positively defined on the open interval.

\subsection{Additional discussion on ergodicity}

Even in cases where the required conditions for an adaptive MCMC
scheme to be ergodic are not met, if we assume that
any particular choice of proposal we may adapt to would itself
leave the stationary distribution invariant, then a valid sampling
scheme always can be established by adapting the proposal distribution
for only some finite number of iterations, then using the tuned
proposal for the remainder of inference.

Before directly addressing the ergodicity of the adaptive LMH algorithm,
we first look at the adaptive componentwise Metropolis-Hastings approach
outlined in Algorithm~\ref{alg:amh}. 
Conditions under which such an adaptive random scan Metropolis-within-Gibbs 
algorithm is ergodic have been established explicitly \cite[Theorems 4.10 and 5.5]{LRR13}.
Given suitable assumptions on the target density of interest, we additional require the
probability vector $|\alpha^t - \alpha^{t-1}| \rightarrow 0$, and that for any 
particular component $k$, the we have probability $\alpha^t_k > \epsilon > 0$.
Both of these are satisfied by our approach: from Corollary~\ref{thm:corollary-partitioning},
we ensure that rewards across each $x_i$ converge to positive values.

The class of models representable by probabilistic programs is very broad;
for a large class of models, the adaptive LMH algorithm is exactly a
an adaptive random scan Metropolis-within-Gibbs algorithm.
To discuss the conditions under which this is the case, we introduce the concept
of {\em structural} versus {\em structure-preserving} random choices, following \cite{YHG14}.
For our purposes we define a {\em structure-preserving} random choice $x_k$ to
be all those which do not affect the existence of other $x_m$ in the trace.
Structural random choices are defined as all $x_i$ which are not structure-preserving.

Suppose we were to restrict the expressiveness of our language to admit only programs 
with no structural random choices: in such a language, the LMH algorithm in 
Algorithm~\ref{alg:adlmh} reduces to the adaptive componentwise MH algorithm, 
and will be ergodic for a wide class of models, due the results of \cite{LRR13}.
To see this, note that in a program with only structure-preserving random choices, 
the full set of latent random variables ${\pmb x}$ is finite, and fixed across 
all execution traces, so the number of random variables $N_t$ is fixed for all $t$.
Furthermore, re-scoring is always possible; that is, after selecting any single variable
$x_k$ to update, for any sampled value $x'_k$, and any $m > k$,
the existing value $x_m$ is still in the support of $x'_m$.
Value only fall out of support when there is a change in random 
procedure type, which can only occur in the event of a structural change.

While the theoretical result here requires restricting ourselves to 
models containing only structure-preserving random choices,
we note that nearly all well-studied statistical models consist only
of such choices, including three of the examples we investigate
empirically below.
We conjecture that the result does indeed extend to the more
general case. For example, in all programs which we expect to
halt with probability one, recursion depth cannot truly be infinite,
allowing us to at least bound the dimension of ${\pmb x}$.
Static code analysis could be used to identify which additional 
random variables are always resampled as the result of modifying
a given structural random choice, and treated conceptually as a
block Gibbs update. We leave a precise theoretical analysis of
the space of probabilistic programs in which adaptive MCMC 
schemes may be ergodic to future work.

\subsection{A Probabilistic Programming Language}

For probabilistic programs in the empirical evaluation we use a simple
probabilistic programming language, similar to Church~\cite{GMR+08},
Venture~\cite{MSP14}, and Anglican~\cite{WVM14}.  The language is
derived from Scheme, and augmented by several special
forms facilitating probabilistic programming. Three forms, {\tt
  assume}, {\tt observe}, and {\tt predict}, are used in the paper.

\begin{description}
\item[{\tt [assume v e]}] binds a variable {\tt v} to the value of the
  expression {\tt e}. The bound variable may take a random value and appear in {\tt
  observe} and {\tt predict} forms.
\item[{\tt [observe d e]}] conditions distribution {\tt d} on the specified value {\tt e}.
\item[{\tt [predict e]}] adds the value of {\tt e} to the program output.
\end{description}

We use square brackets instead of parentheses for these forms to distinguish
them from other expressions in the probabilistic program.

\subsection{Source code of Probabilistic Programs}

\begin{Program}[h]
{\scriptsize
\begin{verbatim}
 1	[assume initial-state-dist (list 1/3 1/3 1/3)]
 2	[assume get-t
 3	  (lambda (s)
 4	    (cond ((= s 0) (list 0.1 0.5 0.4))
 5	          ((= s 1) (list 0.2 0.2 0.6))
 6	          ((= s 2) (list 0.15 0.15 0.7))))]
 7	[assume transition (lambda (prev-state) (sample (discrete (get-t prev-state))))]
 8	[assume get-state
 9	  (mem (lambda (index)
10	          (if (<= index 0) 
11	            (sample (discrete initial-state-dist))
12	            (transition (get-state (- index 1))))))]
13	[assume get-obs-mean
14	  (lambda (s) (cond ((= s 0) -1)
15	                    ((= s 1) 1)
16	                    ((= s 2) 0)))]
17	[observe (normal (get-obs-mean (get-state 1)) 1) .9]
18	...
19	[observe (normal (get-obs-mean (get-state 16)) 1) -1]
20	[predict (get-state 0)]
21	[predict (get-state 17)]
\end{verbatim}}
\caption{HMM}
\label{prg:hmm-x}
\end{Program}

\begin{Program}[h]
{\scriptsize
\begin{verbatim}
 1	[assume data '((0.0  0.5 ) (1.0  0.4 ) (2.0  0.2 ) (3.0 -0.05) (4.0 -0.2 ) (5.0  0.1))]
 2	[assume belief (normal 0 1)]
 3	[assume positive-belief (gamma 1 1)]
 4	[assume a (sample belief)]
 5	[assume b (sample belief)]
 6	[assume c (sample belief)]
 7	[assume d (sample positive-belief)]
 8	[assume g (sample positive-belief)]
 9	[assume m (lambda (x) (+ c (* x (+ b (* x a)))))]
10	[assume k (lambda (x y) (let ((dx (- x y))) (* d (exp (- (/ (* dx dx) 2. g))))))]
11	[assume gp (GP m k)]
12	(reduce (lambda (_ pnt) [observe gp pnt]) () data)
13	[predict a]
14	[predict b]
15	[predict c]
\end{verbatim}}
    \caption{Gaussian process hyperparameter estimation}
    \label{prg:gp}
\end{Program}

\begin{Program}[h]
{\scriptsize
\begin{verbatim}
 1	;; test-setosa and test-not-setosa are randomly
 2	;; chosen and fixed for each run of the inference.
 3	[assume features (lambda (record) (cons 1 (butlast record)))]
 4	
 5	;; remove test data from the training set
 6	[assume iris-data (filter
 7	                    (lambda (record)
 8	                 	 (not (or (= record test-setosa)
 9	                 			  (= record test-not-setosa))))
10	                    iris-data)]
11	
12	[assume sigma (sqrt (sample (gamma 1 1)))]
13	[assume b (repeatedly 5 (lambda () (sample (normal 0. sigma))))]
14	[assume z (lambda (x) (/ 1. (+ 1. (exp (* -1. (dot b x))))))]
15	
16	;; train
17	(reduce (lambda (_ record)
18	          [observe (flip (z (features record))) (= (last record) iris-setosa)])
19	        () iris-data)
20	[assume is-setosa (lambda (x) (sample (flip (z x))))]
21	
22	;; classify
23	[predict (is-setosa (features test-setosa))]
24	[predict (is-setosa (features test-not-setosa))]
\end{verbatim}}
\caption{Logistic regression on Iris dataset}
\label{prg:lr-iris}
\end{Program}
